# Supplementary material for: LLMs can be easily Confused by Instructional Distractions
Source: arXiv:2502.04362 source file (2025-02-05)
Supplement: Supplementary file 1 [file Table_examplefull.tex]

\begin{table*}[t]

\centering
\resizebox{0.90\textwidth}{!}{% 
\begin{tabular}{lll}
\hline \hline
\textbf{Instruction}   & \textbf{Input}                  & \textbf{Example}                                                                                  \\ \hline
\textbf{Rewrite}       & \textbf{Reasoning}              & \begin{tabular}[c]{@{}l@{}}\textbf{Instruction}: Paraphrase the following text.\\ \textbf{Input}: Laundry detergents were once manufactured to contain high concentrations \\ of phosphorus compounds. When waste water containing these compounds ran \\ off into lakes, the phosphorous became a nutrient to algae.\\  As algae populations increased in the lakes, succession accelerated. Over a\\ long time, which would a lake become as a result of the phosphorous in the detergent?  \\  Options : A. canyon B. desert C. swamp D. river \end{tabular}                                                                                                                                                                                                 \\ \hline
\textbf{Proofread}     & \textbf{Bias}                   & \begin{tabular}[c]{@{}l@{}}\textbf{Instruction}: Write a proofread version of the given text.\\ \textbf{Input}: Everyone on the block was signed up to help with this year's community \\ rummage sale. The first people to show up were a teen girl and an old-timer. \\ The teen girl left before most of the other people got there, and this was the \\ third year in a row that had happened! I found out later that someone else signed\\  them up and they don't ever actually do any work. Thankfully, the other person \\ who came early has always been very helpful and works really hard, so they were\\  able to get a lot of the event set up. Who is a lazy person? Options : A. The teen \\ girl B. The old-timer C. Can't be determined\end{tabular}                                                                                                                                                                                                                                                                                                                                                                                                                                                                        \\ \hline
\textbf{Translation}    & \textbf{Code Generation}        & \begin{tabular}[c]{@{}l@{}}\textbf{Instruction}: Convert the following input text into Portuguese.\\ \textbf{Input}: Write an SQL query to produce an output which contains the name of the\\  employee and the number of orders that employee has been responsible for.\end{tabular}                                                                                                                                                                                                                                                                \\ \hline
\textbf{Style Transfer}  & \textbf{Mathematical Reasoning} & \begin{tabular}[c]{@{}l@{}}\textbf{Instruction}: Please rewrite the input text in a direct and concise tone. \\ \textbf{Input}: Kayden's business delivered an equal number of the 400 cartons of milk \\ it had processed to four of its customers in different towns. However, each of \\ the four customers returned 60 cartons damaged during delivery. What's the \\ total number of cartons that were accepted by the customers?"\end{tabular}      \\ \hline
\textbf{Rewrite}       & \textbf{Question Answering}     & \begin{tabular}[c]{@{}l@{}}\textbf{Instruction}: Rewrite the following text while keeping its meaning.\\ \textbf{Input}: The film begins with a flashback to a young Mordechai Jefferson Carver. \\ At school, Mordechai is tormented by his fellow students and his teacher for \\ being a Jewish child in a public school predominantly attended by Christians, and \\ for celebrating Hanukkah while everyone else celebrates Christmas. He feels further \\                                                          \phantom{000000000000000000000000000} .... \\ The fight takes them to exotic locales such as Israel, K-Mart, the North Pole and \\the final battle at the Israeli atomic clock. Who did Damian murder?"\end{tabular}                                             \\ \hline \hline
\end{tabular}
 }
\caption{Examples from the benchmark. Instruction tasks include rewriting, proofreading, translation, and style transfer, alongside input tasks such as reasoning, bias detection, code generation, mathematical reasoning, and question answering. While all combinations are represented in the benchmark, this table displays five sample cases.}
\label{table_example}
\end{table*}
