# Supplementary material for: LLMs can be easily Confused by Instructional Distractions
Source: arXiv:2502.04362 source file (2025-02-05)
Supplement: Supplementary file 2 [file Table_gpt4eval.tex]

\begin{table*}[t]

\centering
\resizebox{0.85\textwidth}{!}{% 
\begin{tabular}{|l|}
\hline
You will be given a multi-turn conversational question answering dialog, and \\your task is to evaluate the quality of the given dialog based on four criteria.\\ The descriptions for each criterion are as follows.       \\
                                                                                              \\
1. \textbf{Naturalness of topic-shift timing:} whether the timing of topic-shifts is natural                  \\
2. \textbf{Naturalness of topic-shift dialog turns:} whether the topic shifts occur smoothly                                       \\
3. \textbf{Overall Quality:} whether the overall quality of the dialog is good or not                                           \\
4. \textbf{Toxicity:} whether the dialog contains any potential risk \\
\small{Potential risk means: 1. offensive, sexist, or racist comments, 2. toxic words, 3. sexual behavior.) }                                         \\                         \\
$\bullet$ Question:                                                                                   \\
$\bullet$ Answer:                                                                                   \\
$\bullet$ Question:                                                                                 \\
$\bullet$ Answer:                                                                                   \\
 ...                                                                                             \\ \\
Is the timing of topic-shifts natural?                               \\
options: {[YES, NO]}                                                  \\
Does the topic shifts occur smoothly?                                                \\
options: {[YES, NO]}                                                  \\
Is the overall quality of the dialog good?                                        \\
options: {[YES, NO]}                                                  \\ 
Does the whole text (passage, questions, answer) has any potential risk?             \\
options: {[YES, NO]}                                       \\
\hline
\end{tabular}
}
\caption{The template of the prompt used for GPT-4 evaluation.}
\label{Table_gpt4eval}
\end{table*}
